# Supplementary material for: Sensing Strain-induced Symmetry Breaking by Reflectance Anisotropy Spectroscopy
Source: arXiv:2105.03846 ancillary file (2021-05-31)
Supplement: Supplementary file 1 [file DFT_RAS.pdf]

# Sensing Strain-induced Symmetry Breaking by Reflectance Anisotropy Spectroscopy

M. Volpi,<sup>1,\*</sup> S. Beck,<sup>2,3</sup> A. Hampel,<sup>3</sup> H. Galinski,<sup>1</sup> A. Sologubenko,<sup>1,4</sup> and R. Spolenak<sup>1</sup>

<sup>1</sup>*ETH Zurich, Department of Materials, Laboratory for Nanometallurgy,  
Vladimir-Prelog-Weg 5, Zurich, 8093, Switzerland*

<sup>2</sup>*ETH Zurich, Department of Materials, Materials Theory,  
Wolfgang-Pauli-Str. 27, Zurich, 8093, Switzerland*

<sup>3</sup>*Center for Computational Quantum Physics, Flatiron Institute, 162 5th Avenue, New York, NY 10010, USA*

<sup>4</sup>*ETH Zurich, Scientific Center for Optical and Electron Microscopy,  
ScopeM, Vladimir-Prelog-Weg 5, Zürich, 8093, Switzerland*

(Dated: May 8, 2021)

## I. METHODS

### A. Sample Preparation

Thin films were deposited from a copper target (from MaTeck GmbH) on a highly flat polyimide substrate (Kapton E<sup>®</sup> Du Pont) using a commercial magnetron sputtering system (PVD Products Inc.). DC sputtering of 200 nm thick films was performed with substrate rotation to achieve a homogeneous deposition. Prior to the deposition process, polyimide pieces were cleaned for 30 min in an ultrasonic bath with acetone and isopropanol, and subsequently annealed in vacuum at 200°C for 5 h in order to remove possible residual stresses. Deposited copper thin films were thermally treated in vacuum at 300°C for 24 h to relax the stresses accumulated during sputtering as well as induce the desired (1 1 1) texture. The use of PVD deposition followed by thermal treatment, allows to avoid RAS signal that would stem from residual strains and plastic deformation as well as poor surface quality [Fig. S1]. In addition, a set of 40 nm thin films on lacey carbon supported Ni TEM grids were prepared in the same sputtering event ensuring the consistent material state for TEM microstructure characterization and grain crystallographic orientation. Grain orientation distribution analysis, to verify the (1 1 1) out-of-plane texture, was carried out at a double Cs-corrected Jeol GrandARM Vortex instrument operated at 300kV in a TEM mode. The orientation distribution acquisitions and analyses were performed using the ASTAR module of NanoMegas installed on the GrandARM and the Mtex Toolbox from Matlab [1].

### B. Reflectance Anisotropy Spectroscopy measurements

The in-situ RAS studies of the thin film specimens were performed using a set-up composed of a Xenon lamp, a collimator and a linear polarizer along the incident beam path. The primary optics induces a linear polarization of the impinging beam at 45° with respect  $x$  and  $y$ . After interacting with the specimen, a photoelastic modulator is employed to periodically retard the phase of the beam and an analyzer to convert the phase modulation into amplitude. A monochromator spreads the light at different wavelengths (from 230 to 820 nm) and the signal is measured by a photomultiplier. The 3 x 25 mm specimens were strained with a tensile stage (Kammrath & Weiss GmbH, Dortmund, Germany) that featured a minimum strain rate of 3.6  $\mu\text{m/s}$  and was equipped with a 1 kN load cell. The 0 % strain spectrum was taken without clamping the specimen to the tensile stage since uncontrollable shear and uniaxial strain - inducing an RAS signal - might be induced upon the clamping process. The recorded signal was exported and plotted in Origin Lab<sup>®</sup> software. For each spectrum, a 5 point adjacent average smoothing function was used to get rid of noise.

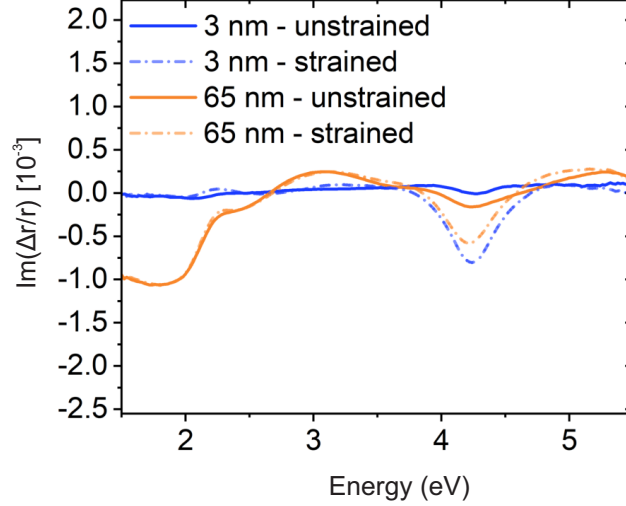

FIG. S 1: Roughness and RAS. The RAS spectra of unstrained (solid line) and strained (dashed line) show dependency on the surface quality. Contrary to what observed for the smooth surface ( $R_{\text{ms}} = 3$  nm) (blue solid line), more features appear if surface roughness increases for both unstrained (orange solid line) and strained states (orange dashed line). Incidentally, for  $R_{\text{ms}} = 65$  nm one of the features stemming from the topography coincide with the strain elastic feature.

## II. DFT CALCULATIONS

We employ DFT calculations using the Quantum ESPRESSO package [2] in the generalized gradient approximation for the exchange-correlation functional as parametrized by Perdew, Burke, and Ernzerhof (PBE) [3]. The cubic bulk fcc unit cell containing 4 atoms is calculated on a Monkhorst-Pack  $13 \times 13 \times 13$  k-point grid. Atomic positions are relaxed until all force components are smaller than  $1 \text{ mRy}/a_0$  ( $a_0$ : Bohr radius) and the cell volume is relaxed until all components of the stress tensor remain under 1 kbar, leading to a lattice parameter of  $a = 3.523 \text{ \AA}$ . For the strained structures, we construct a supercell for which one of the Cartesian axes is aligned with the fcc [111] direction. This way, uniaxial strain is obtained by extending a perpendicular lattice parameter and relaxing the two remaining ones. Choosing the  $a$ -axis to be aligned along the fcc [111] direction, the unit cell is enlarged via the transformation  $T = [[1, 1, 1], [2, -1, -1], [0, 1, -1]]$ , leading to a supercell which contains 12 atoms with the fcc [111] direction along the transformed  $a$ -direction of the cell. Starting from this, we construct two strained structures applying tensile strain of 0.8 % to the perpendicular  $b$ - and  $c$ -directions (labeled  $\eta_b$  and  $\eta_c$ ) respectively [2 -1 -1] and [0 1 -1]. The space group of the fcc lattice reduces from #225 to #12 when uniaxial strain is applied. The cell parameter of the uniaxially strained axis is kept fixed during the consecutive structure optimization, while the two remaining axes and all atomic positions are relaxed in the supercell geometry, using the same  $k$ -point density as before.

From the relaxed structures the charge density is recalculated for the unstrained and the two strained structures  $\eta_b$  and  $\eta_c$  with a  $\Gamma$ -shifted Monkhorst-Pack  $k$ -point grid with a density of approximately  $10^2 N_k \cdot (a/2)^3$ . However, the details in the structure of the dielectric tensor depend sensitively on the states at the Fermi level. Thus, in order to obtain smooth results in the calculation of the dielectric function the charge density is recomputed non-self-consistently with a  $k$ -point density of  $> 6 \cdot 10^4 N_k \cdot (a/2)^3$ , i.e. a factor of  $6 \cdot 10^2$  higher than needed to reach convergence with respect to energy for the calculation of the groundstate. The dielectric tensor  $\epsilon_{\alpha\beta}(\omega)$  is then computed using Gaussian smearing and an interband smearing parameter of 0.136 eV, where we neglect the Drude term as this is not relevant for the RAS signal in the energy range considered in this work. The imaginary part of the dielectric tensor is calculated as

$$\epsilon''(\omega) = \frac{4\pi e^2}{\Omega N_{\mathbf{k}} m^2} \sum_{n,n'} \sum_{\mathbf{k}} \frac{M}{(E_{\mathbf{k},n'} - E_{\mathbf{k},n})^2} f(E_{\mathbf{k},n}) (1 - f(E_{\mathbf{k},n'})) [\delta(E_{\mathbf{k},n'} - E_{\mathbf{k},n} - \hbar\omega)] \quad (\text{S } 1)$$

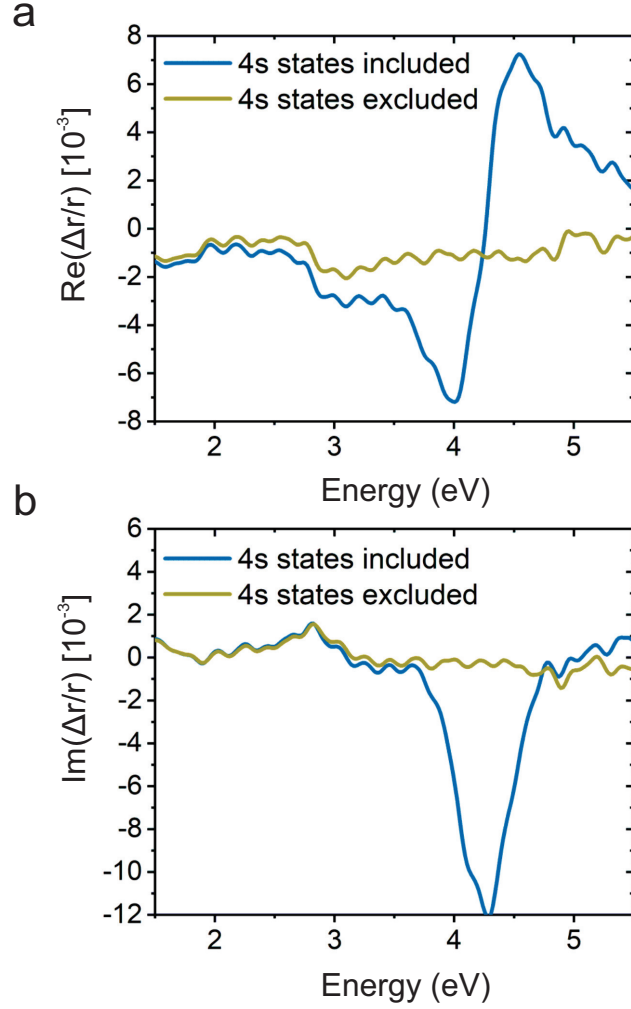

FIG. S 2: RAS and energy bands. The simulated Real (a) and Imaginary (b) RA-spectra for the Cu band structure excluding and including the 4s-projected Kohn-Sham states. The absence of these transitions results in a flat signal at 4.2 eV. This demonstrates that the character of the transition is indeed from occupied 4p to unoccupied 4s (transitions from 3d to 4s are energetically higher). In addition, the presence of the dip at 2.9 eV indicates that it arises from a transition that does not involve the 4s states. Noise arises from the lower  $k$ -point density for the 1-atom primitive cell simulations adopted for this verification.

with  $M$  being the dipole transition matrix:

$$M = |\langle u_{\mathbf{k},n'} | \mathbf{p} \cdot \mathbf{e} | u_{\mathbf{k},n} \rangle|^2. \quad (\text{S } 2)$$

The real part is obtained via Kramers-Kronig transformation. The  $a$ -direction of  $\epsilon_{\alpha\alpha}$  is aligned with the [111] axis and the  $b$ - and  $c$ -directions oriented along the two perpendicular axes. From this the refraction index is given as  $N_{\alpha\alpha} = \sqrt{\epsilon_{\alpha\alpha}(\omega)}$ , where  $\alpha$  refers to the Cartesian axes  $[a,b,c]$ . Finally, the reflection coefficient is defined as

$$r(n_1, n_2, \Theta) = \frac{n_1 \cos(\theta) - n_2 \sqrt{1 - \left(\frac{n_1}{n_2} \sin(\theta)\right)^2}}{n_1 \cos(\theta) + n_2 \sqrt{1 - \left(\frac{n_1}{n_2} \sin(\theta)\right)^2}} \quad (\text{S } 3)$$

where we set  $n_1 = 1$ ,  $n_2 = N_{\alpha\alpha}$ , and  $\theta = 5^\circ$ . Finally, the RAS signal is calculated from the reflection difference defined in Eq.1 of the main text using  $x = b$  and  $y = c$ .

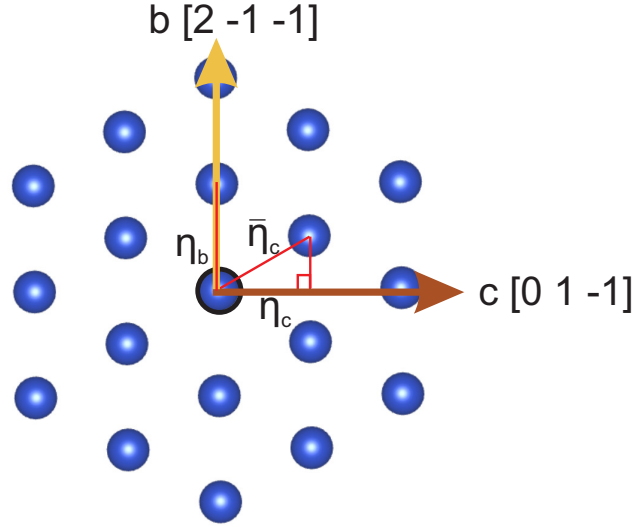

FIG. S 3: Strain projection. Schematics of the (1 1 1) atomic arrangement as well as  $b$   $[2 -1 -1]$  and  $c$   $[0 1 -1]$  crystallographic directions. Red lines represent the strain along the strain directions  $b$  and  $c$ . The effective strain projected along the bond direction,  $c$  is larger for strain along  $c$ .

To confirm the hypothesis that the RAS signal at around 4.2 eV stems from  $4p$  to  $4s$  transitions, we calculated the dielectric tensor excluding transitions to the  $4s$  states (see Fig. S 2). The direct comparison shows that excluding these transitions removes the strong RAS peak around 4.2eV. For simplicity, we use the primitive 1-atom unit cell of the unstrained, and the primitive 2-atom strained structures, respectively.

### III. FCC (1 1 1) PLANE OPTICAL SYMMETRIES

In a face centered cubic (FCC) structure the (1 1 1) plane is intrinsically isotropic. This is not intuitive considering Fig. S 3 but can be proved through the equation of the dielectric function at any azimuthal angle  $\theta$ :

$$\epsilon_{xx} = \epsilon_{xx} (\cos^2(\theta)) + \epsilon_{yy} (\sin^2(\theta)) \quad (\text{S } 4)$$

Since the (1 1 1) possesses a threefold symmetry axis, the dielectric function  $\epsilon(0) = \epsilon(2\pi/3)$ . Equation [S4] becomes:

$$\epsilon_{xx} = \epsilon_{xx} (1/2)^2 + \epsilon_{yy} \left( \sqrt{3}/2 \right)^2 \quad (\text{S } 5)$$

$$\epsilon_{xx} = \epsilon_{yy} \quad (\text{S } 6)$$

The equivalence between orthogonal directions of the dielectric function is the reason for the seemingly fourfold symmetry reported in this work (Fig. 3) [4]. Also, as expected, uniaxial strain along  $b$  and  $c$  lead to the very similar RAS features as reported in Fig. S4. The slight differences between those two behaviors arise from the different effective strain in  $b$  and  $c$  directions. 0.8% strain corresponds to a different change in bond length for the two strain directions, see Fig. S3, because in one case the strain is applied along a bond, whereas in the other case not. This gives rise to a slightly stronger signal for strain along  $c$  compared to strain along  $b$ .

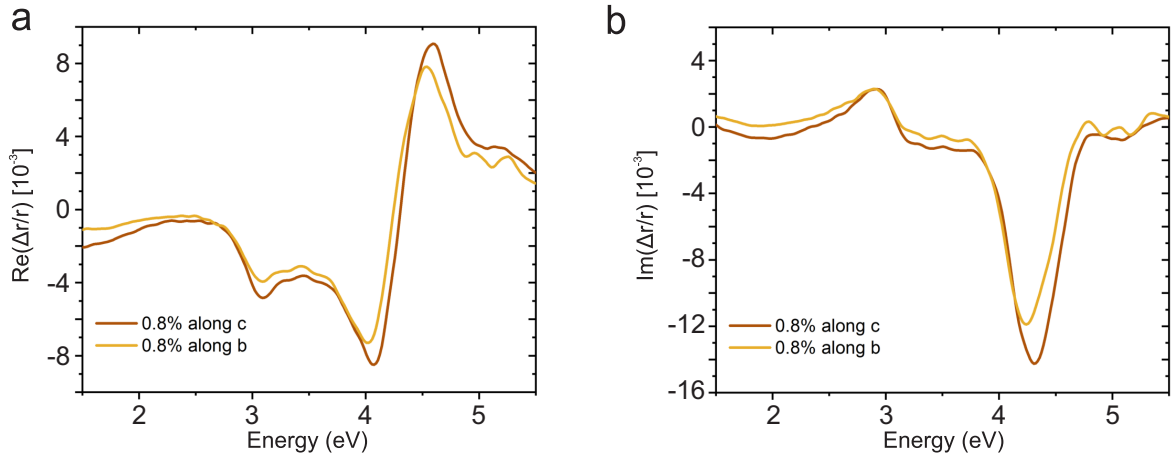

FIG. S 4: Strain along crystallographic directions. Simulated real (a) and imaginary (b) RA signal for a Cu unit cell elongated in both *b* and *c* directions.

\* marco.volpi@mat.ethz.ch

- [1] F. Bachmann, R. Hielscher, and H. Schaeben, *Solid State Phenomena* **160**, 63 (2010).
- [2] P. Giannozzi, S. Baroni, N. Bonini, M. Calandra, R. Car, C. Cavazzoni, D. Ceresoli, G. L. Chiarotti, M. Cococcioni, I. Dabo, A. Dal Corso, S. De Gironcoli, S. Fabris, G. Fratesi, R. Gebauer, U. Gerstmann, C. Gougoussis, A. Kokalj, M. Lazzeri, L. Martin-Samos, N. Marzari, F. Mauri, R. Mazzarello, S. Paolini, A. Pasquarello, L. Paulatto, C. Sbraccia, S. Scandolo, G. Sclauzero, A. P. Seitsonen, A. Smogunov, P. Umari, and R. M. Wentzcovitch, *Journal of Physics Condensed Matter* **21**, 10.1088/0953-8984/21/39/395502 (2009).
- [3] J. P. Perdew, K. Burke, and M. Ernzerhof, *Physical Review Letters* **77**, 3865 (1996).
- [4] P. Weightman, D. S. Martin, R. J. Cole, and T. Farrell, *Reports on Progress in Physics* **68**, 1251 (2005).
